# Supplementary material for: Let Me Speak Freely? A Study on the Impact of Format Restrictions on Performance of Large Language Models
Source: arXiv:2408.02442 source file (2024-10-14)
Supplement: Supplementary file 1 [file appendix.tex]

\subsection{JSON-mode averaged scores}

\begin{table}[t]
\centering
\small
\begin{tabular}{@{}lcccc@{}}
\toprule
\textbf{Dataset} & \textbf{GPT3.5T} & \textbf{Flash} & \textbf{LLaMA3} \\
\midrule
LastLetter & 1.78 (0.3) & 0.67 (0.5) & 7.56 (2.7) \\
GSM8K & 29.87 (0.8) & 47.78 (3.1) & 65.38 (1.3) \\
\midrule
MultiFin &66.00 (1.3) & 66.79 (0.4) & 54.82 (1.5)\\
Sports & 76.82 (0.9) & 77.79 (0.4) & 72.08 (2.6) \\
Task 280 & 78.07 (2.3) & 67.19 (4.1) & 74.57 (2.0)\\
DDXPlus & 51.87 (2.8) & 84.92 (2.1) & 22.59 (0.1)\\
\bottomrule
\end{tabular}
\caption{Applying JSON-mode to all 6 datasets and found}
\label{tab:json_mode}
\end{table}
