# Supplementary material for: Let Me Speak Freely? A Study on the Impact of Format Restrictions on Performance of Large Language Models
Source: arXiv:2408.02442 source file (2024-10-14)
Supplement: Supplementary file 2 [file other_prompt_format.tex]

\noindent \textbf{Hybrid method} In this setting, we explore a hybrid method between complex reasoning and only format the final answer in targeted format.

\noindent \textbf{2 stage text-to-format} We decompose the reasoning and formatting into a 2 step process, where the LLM first reasons and answers in natural language followed by a second instruction to reformat it into our target format schema.
